# Supplementary material for: Preconditioned Least-Squares Petrov-Galerkin Reduced Order Models
Source: arXiv:2203.12180 source file (2022-03-23)
Supplement: Supplementary file 1 [file appendix.tex]

\section{Appendix}
\label{sec:appendix}

This is the appendix (if necessary; if not, remove).
